# Supplementary material for: Energy-optimal Design and Control of Electric Powertrains under Motor Thermal Constraints
Source: arXiv:2111.07711 source file (2022-04-12)
Supplement: Supplementary file 1 [file appendix1.tex]

\section{Alternative Figures}\label{sec:AltFig}

\begin{figure}[h!]	
	\centering
	\includegraphics[trim=0.95cm 0cm 1.45cm 0cm,clip=true,  width=\columnwidth]{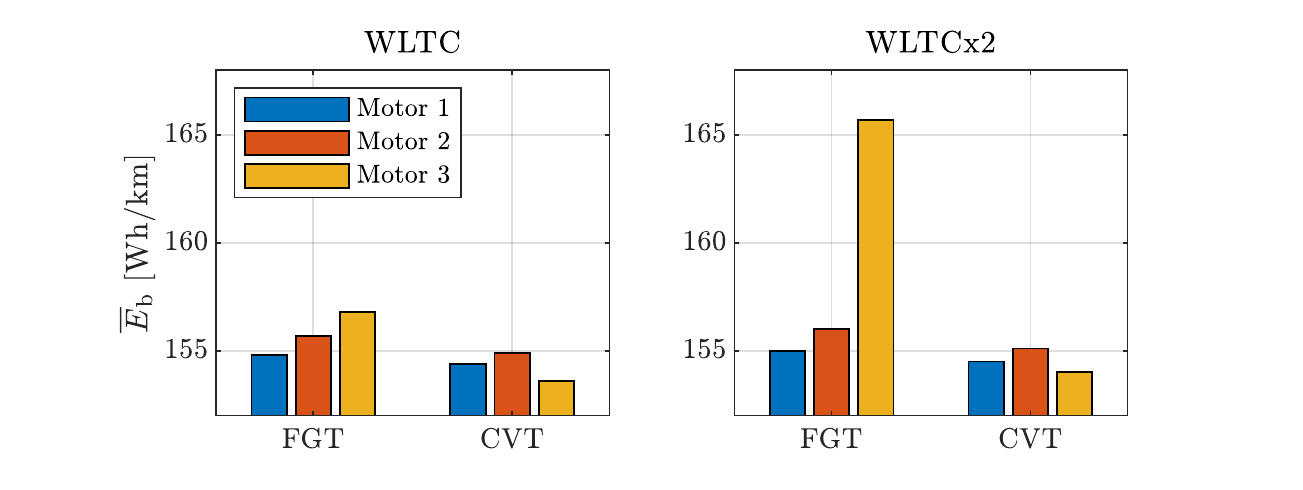}
	%	\caption{ The resulting powers, temperatures for an electric powertrain equipped with Motor 3, CVT and simulated over the WLTCx2 cycle. }
	\caption{@Mauro. As we discussed yesterday, the energy consumption of CVT equipped powertrains is not decreasing. Rather they show random behaviour. I was not sure if this can be included in the results. Let me know.}
	\label{fig:BarGraph_Paper1}
\end{figure}%
%
%\begin{figure}[h!]	
%	\centering
%	%\includegraphics[trim=1.85cm 1.85cm 2cm 1.95cm,clip=true, width=\columnwidth]{img/AR751_CVT_WLTP_Rep2_4.pdf}
%	\includegraphics[trim=0.95cm 0cm 1.45cm 0cm,clip=true,  width=\columnwidth]{img/BarGraph_Paper2.pdf}
%	%	\caption{ The resulting powers, temperatures for an electric powertrain equipped with Motor 3, CVT and simulated over the WLTCx2 cycle. }
%	\caption{Same figure but monochromatic}
%	\label{fig:BarGraph_Paper2}
%\end{figure}%
